# Supplementary material for: Spiral spin liquid in a frustrated honeycomb antiferromagnet: A single-crystal study of GdZnPO
Source: arXiv:2503.12396 source file (2025-03-16)
Supplement: Supplementary file 1 [file Supplementary_r1.pdf]

*Supplementary material*

# Spiral spin liquid in a frustrated honeycomb antiferromagnet: A single-crystal study of GdZnPO

Zongtang Wan,[1,*] Yuqian Zhao,[1,*] Xun Chen,[1] Zhaohua Ma,[1] Zikang Li,[1] Zhongwen Ouyang,[1] and Yuesheng Li[1,†]

[1] *Wuhan National High Magnetic Field Center and School of Physics, Huazhong University of Science and Technology, 430074 Wuhan, China*

We present here:

I. Sample synthesis and characterization.

Fig. S1. Typical crystal and x-ray diffraction patterns.

Fig. S2. Specific heat measurements.

Fig. S3. Electron spin resonance spectra.

Tab. S1. Single-crystal structure refinement.

II. Spiral spin-liquid ansatz.

III. Monte Carlo simulations and low-energy topological defects.

Fig. S4. Calculated spin structure factors at various temperatures.

Fig. S5. Calculated spin configuration projected onto the $ab$ plane for all six sublattices.

Fig. S6. Local momentum vortices on all six sublattices.

Fig. S7. Calculated spin configuration on the $A$ and $B$ sublattices and on the entire honeycomb lattice, and entropy increase.

* These authors contributed equally to this work

† yuesheng_li@hust.edu.cn

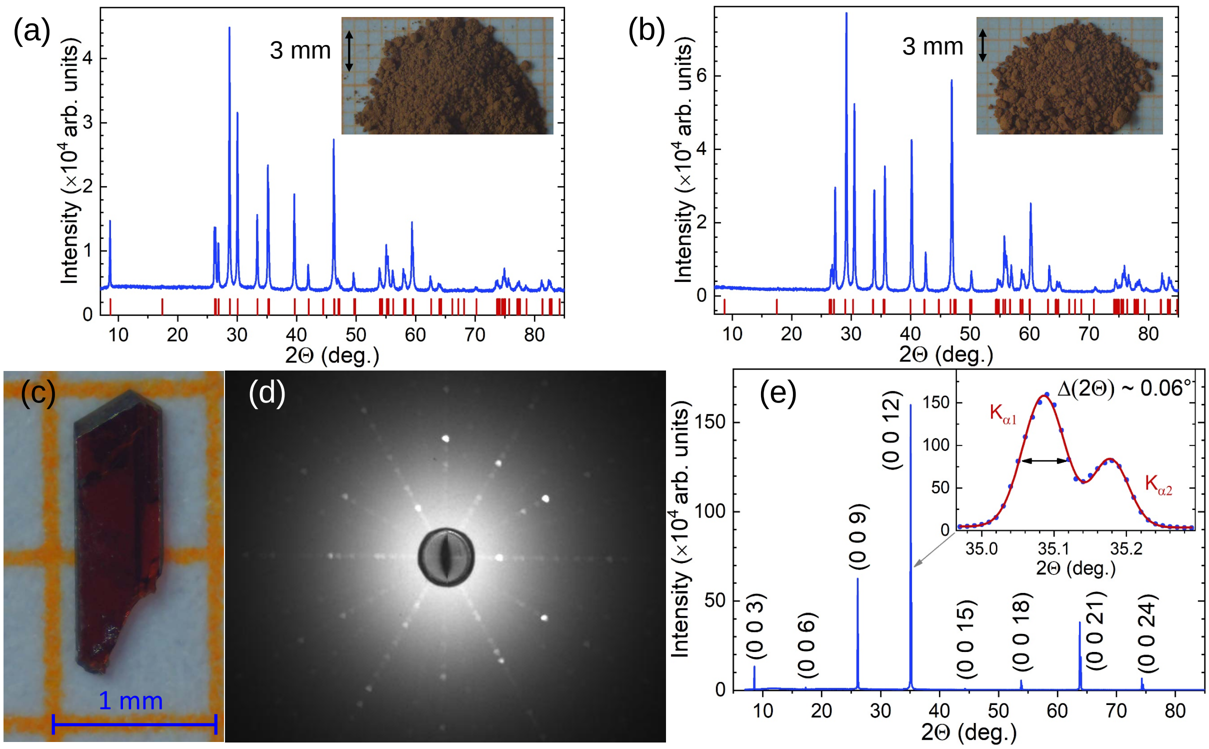


FIG. S1. Powder XRD patterns of precursor GdZnPO (a) and YZnPO (b), with red bars indicating calculated reflection positions. Insets show the respective powders. (c) Typical as-grown single crystal of GdZnPO. (d) Laue XRD pattern on the *ab* plane. (e) XRD pattern on the *ab* plane. Inset: Zoomed view of the (0 0 12) reflection with a two-Gaussian fit; the fitted full width at half maximum is listed.

## I. SAMPLE SYNTHESIS AND CHARACTERIZATION

We grew high-quality single crystals of GdZnPO in two steps. First, polycrystalline GdZnPO precursor was synthesized via a solid-phase method using stoichiometric mixtures of gadolinium (99.9%, Aladdin), zinc oxide (99.99%, Aladdin), and red phosphorus (99.999%, Alfa Aesar). The materials were mixed, pressed into pellets in an argon-filled glove box, and sealed in vacuum ($\leq 1.0\times10^{-5}$ bar) in quartz tubes. The tubes were heated to 950°C for three days, yielding brown GdZnPO powders [see Fig. S1(a)], confirmed by powder x-ray diffraction (XRD, Cu $K_\alpha$, $\overline{\lambda}$ = 1.5418 Å, Rigaku) for phase purity and air insensitivity. Second, single crystals were grown using the flux method. The GdZnPO powders were mixed with equimolar NaCl/KCl flux in a 1:50:50 mole ratio, sealed in quartz tubes under vacuum, and heated to 1050°C for ten days. The excess flux was removed with highly pure water, and GdZnPO showed water insensitivity at room temperatures.

The as-grown GdZnPO single crystals are reddish-brown and transparent [see Fig. S1(c)]. Laue photographs of the crystals show sharp reflections [LAUESYS_V_674, Photonic Science & Engineering Ltd, see Fig. S1(d)], and the XRD Bragg reflections can be fitted with Gaussian-peak functions, with a full width at half maximum of $\sim$ 0.06°, only slightly larger than the instrumental resolution of 0.05° [see Fig. S1(e)]. These results indicate the high quality of the single-crystal samples. No additional reflections were observed in the XRD patterns, confirming the pure phase of GdZnPO. The structural reflection positions [Fig. S1(e)] yield a lattice parameter $c$ = 30.58(2) Å, consistent with the previously reported value [1]. Furthermore, the GdZnPO crystal structure determined by single-crystal XRD (Mo $K_\alpha$, $\overline{\lambda}$ = 0.71073 Å, XtaLAB mini II, Rigaku) and refinements (Table S1) agrees well with the reference [1].

The powder of the nonmagnetic reference compound YZnPO was synthesized using a similar solid-phase method. Yttrium (99.99%, Aladdin), zinc oxide (99.99%, Aladdin), zinc (99.99%, Aladdin), and red phosphorus (99.999%, Alfa Aesar) were mixed in a molar ratio of 1:0.85:0.19:1.035, following the same procedure as for the GdZnPO powder synthesis. The phase purity of YZnPO was confirmed by powder XRD [see Fig. S1(b)]. The specific heat of YZnPO, shown in Fig. S2(a), represents the lattice contribution and was subtracted from the total specific heat of GdZnPO in the main text.

The specific heat above 1.8 K was measured using a physical property measurement system (PPMS, Quantum Design). The setup for milli-Kelvin specific heat measurements is shown in Fig. S2(b) [2–4]. Temperatures ranging from 53 mK to 1.8 K were achieved using a $^3$He-$^4$He dilution refrigerator (KELMX-400, Oxford Instruments). Ac resistance Bridges & temperature controllers (model 372, Lakeshore) were used to measure thermometer resistances, control the heat sink temperature, and apply

TABLE S1. Structure refinement of the single-crystal XRD data measured at 300 K. Occupancy fractions were set to "1" for all atoms, following the methodology in Ref. [1].

| crystal size used in refinement | 0.11×0.11×0.05 mm |
|---|---|
| space group | $R\bar{3}m$ |
| $a$ ($\equiv b$) | 3.9180(4) Å |
| $c$ | 30.531(3) Å |
| cell volume, $Z$ = 6 | 405.9±0.1 Å$^3$ |
| Gd: $z$ ($x \equiv y \equiv 0$) | 0.38035(8) |
| $U_{11}(\equiv U_{22})$,$U_{33}$,$U_{12}$ ($U_{13} \equiv U_{23} \equiv 0$) | 0.0120(9),0.006(1),0.0060(4) |
| Zn: $z$ ($x \equiv 0$ and $y \equiv 0$) | 0.8038(2) |
| $U_{11}(\equiv U_{22})$,$U_{33}$,$U_{12}$ ($U_{13} \equiv U_{23} \equiv 0$) | 0.019(2),0.017(3),0.009(1) |
| P: $z$ ($x \equiv 0$ and $y \equiv 0$) | 0.1113(5) |
| $U_{11}(\equiv U_{22})$,$U_{33}$,$U_{12}$ ($U_{13} \equiv U_{23} \equiv 0$) | 0.018(4),0.009(6),0.009(2) |
| O: $z$ ($x \equiv 0$ and $y \equiv 0$) | 0.304(1) |
| $U_{11}(\equiv U_{22})$,$U_{33}$,$U_{12}$ ($U_{13} \equiv U_{23} \equiv 0$) | 0.01(1),0.04(2),0.006(5) |
| $h$ range | $-5 \to 5$ |
| $k$ range | $-4 \to 5$ |
| $l$ range | $-42 \to 18$ |
| number of reflections ($I > 0$) | 523 |
| number of reflections ($I > 3\sigma_I$) | 485 |
| $R(F)$ ($I > 3\sigma_I$) | 7.2% |
| $R_w(F)$ ($I > 3\sigma_I$) | 9.6% |

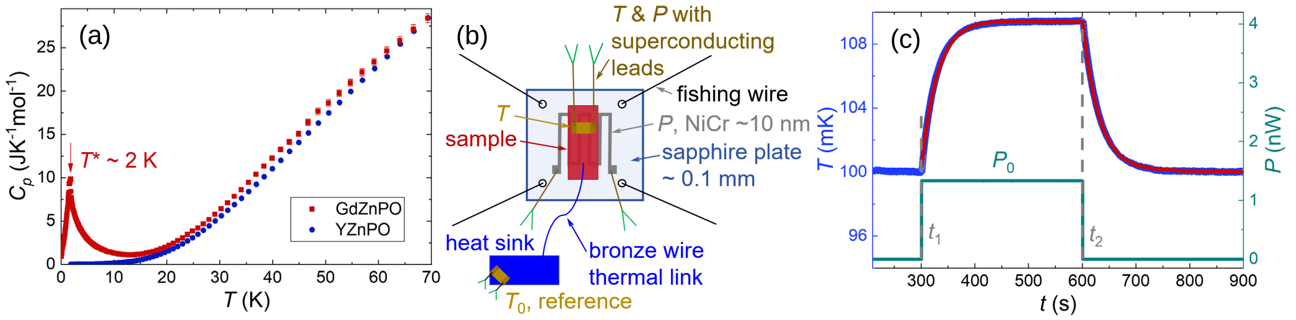


FIG. S2. (a) Specific heat of GdZnPO and YZnPO at 0 T, with the arrow representing the peak temperature $T^* \sim 2$ K. (b) Schematic of the platform used for milli-Kelvin specific heat measurement. (c) Relaxation curve (blue) and heater power (green) for the GdZnPO single crystal at 0 T, with the red line showing a fit to the relaxation data.

an electric current to the sample heater. A $\sim$ 10 nm NiCr layer was deposited on the lower side of a 0.1 mm sapphire plate, serving as the heater. The NiCr heater's resistance is temperature-insensitive, allowing for a perfect square wave of power ($P$) by applying constant current between $t_1$ and $t_2$, as shown in Fig. S2(c). Heater power was measured using 7.5-digit multimeters (DMM7510, Keithley). A plate-like single crystal of GdZnPO (mass, $m$ = 0.98 mg) was mounted on the upper side of the sapphire plate, with the magnetic field applied along the $c$ axis ($H^{\parallel}$). A thin film thermometer (CX-1010-BR, Lakeshore, marked as "$T$") mounted on the upper side of the sample was *in situ* calibrated against a reference thermometer (RX-102B-RS-0.02B, Lakeshore, calibrated down to 20 mK, marked as "$T_0$") at the start of each measurement ($t < t_1$), by turning off the heater ($P$ = 0). The thermal link to the heat sink was provided by a thin bronze wire, adjusted to create quasi-adiabatic conditions. Each thermal relaxation measured for $t > t_1$ can be well fitted by

$$T(t) = \Delta T[1 - \exp(\frac{t_1 - t}{\tau})](t > t_1) - \Delta T[1 - \exp(\frac{t_2 - t}{\tau})](t > t_2) + T_0, \quad (1)$$

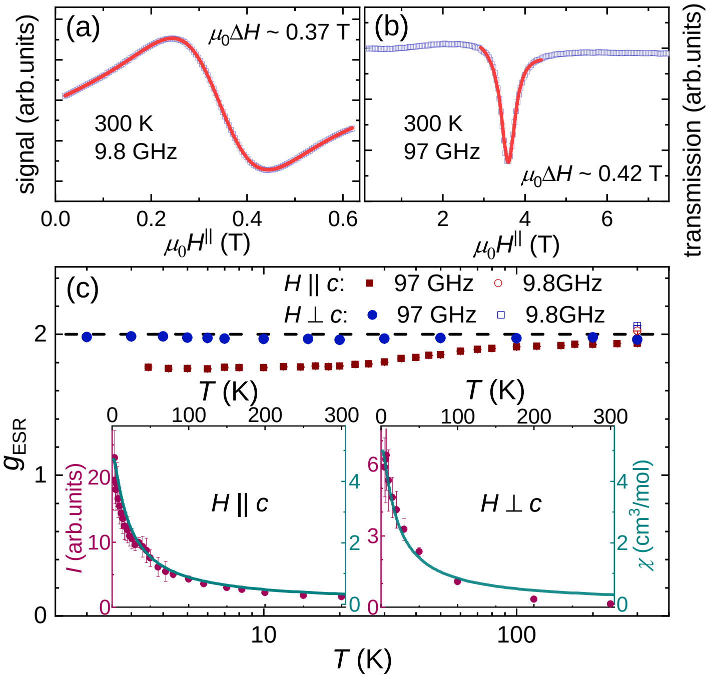


FIG. S3. (a) First-derivative ESR absorption spectrum of GdZnPO measured along the $c$ axis at 300 K and x-band frequencies ($\sim$ 9.8 GHz). The red line shows a first-derivative Lorentzian fit. (b) Pulsed-field ESR absorption spectrum along the $c$ axis at 300 K and 97 GHz, with the red line showing a Lorentzian fit. (c) ESR g factors. Insets compare pulsed-field ESR intensities (scatter) with bulk susceptibilities (lines) measured parallel (left) and perpendicular (right) to the $c$ axis.

where $\Delta T$, $T_0$, and $\tau$ are the fitting parameters. Therefore, the molar specific heat is obtained as

$$C_p(T = T_0 + \frac{\Delta T}{2}) = \frac{M_{\rm m} P_0 \tau}{m \Delta T}, \tag{2}$$

where $M_{\rm m}$ = 269.6 g/mol is the molar mass. For instance, as shown in Fig. S2(c), fitting yielded $\Delta T \sim$ 9.3 mK, $T_0 \sim$ 100.3 mK, and $\tau \sim$ 29.95 s. With the measured $P_0$ = 1.333 nW, we calculated $C_p \sim$ 1.18 JK$^{-1}$/mol at $T \sim$ 105 mK and $\mu_0 H^{||}$ = 0 T.

The first-derivative electron spin resonance (ESR) spectra were collected using a continuous-wave spectrometer (Bruker EMXmicro-6/1) at 300 K and x-band frequencies ($\sim$ 9.8 GHz) on a well-aligned single-crystal sample of GdZnPO ($\sim$ 30.2 mg), with the magnetic field applied parallel and perpendicular to the $c$ axis [3]. Pulsed-field ESR spectra were measured during the field-increasing process at 97 GHz, down to $\sim$ 2 K, on the same sample [5–7]. Despite the frequency increase from 9.8 to 97 GHz, the ESR linewidth ($\mu_0\Delta H$) remains nearly unchanged along the $c$ axis [compare Figs. S3(a) and S3(b)]. This is also observed in spectra measured perpendicular to the $c$ axis, $\mu_0\Delta H^{\perp}$ = 0.36 T at 9.8 GHz and 0.27 T at 97 GHz, at 300 K (see the main text). Therefore, we conclude that $\mu_0\Delta H$ remains $\sim$ 0.27-0.42 T at $\sim$ 300 K for the GdZnPO spin system. The $g$-factor tensor measured at both 9.8 and 97 GHz shows good isotropy, with diagonal $g$ factors approaching the free electron value, $g^{||} \sim g^{\perp} \sim 2$, consistent with the zero orbit angular momentum of $Gd^{3+}$ ($L$ = 0). The slight decrease in $g^{||}$ as temperature cools may be attributed to the formation of easy-plane spin configurations [see Fig. S3(c)]. As shown in the insets of Fig. S3(c), ESR intensities increase with decreasing temperature, following the bulk susceptibilities. These results indicate that GdZnPO remains paramagnetic down to $\sim$ 2 K.

The aligned single-crystal sample of GdZnPO ($\sim$ 30.2 mg) was also used for magnetization ($M$) measurements. Between 1.8 and 300 K, magnetization and susceptibility were measured using a magnetic property measurement system (Quantum Design) up to 7 T. At 1.9 and 4.2 K, magnetization was measured up to 14 T with a vibrating sample magnetometer in a PPMS. For measurements between 0.03 and 1.9 K, a high-resolution Faraday force magnetometer in the $^3$He-$^4$He dilution refrigerator was used, with 13 mg of aligned crystals. Main magnetic fields ($\mu_0|H^{||}| \leq$ 12 T) and field gradients ($\mu_0|{\rm d}H^{||}/{\rm d}z| \leq$ 10 T/m) were generated by superconducting coils (in INTA-LLD-S12/14, Oxford Instruments). The electric capacitance ($c_{\rm e}$) was measured using a $f$ = 1 kHz ultra-precision capacitance bridge (AH-2500A, Andeen-Hagerling) with the three-terminal method [8–10]. The parallel loss $l_{\rm p} \sim -0.036$ nS was negligible, and the parallel capacitance $c_{\rm p} \sim$ 3.4 pF or series capacitance $c_{\rm s}$ was nearly equal to $c_{\rm e}$, with $c_{\rm s}/c_{\rm p} - 1 = l_{\rm p}^2/(2\pi f c_{\rm p})^2 \sim 2.8\times10^{-6}$, comparable to the noise-to-signal ratio of $c_{\rm p}$ ($\sim 1.5\times10^{-6}$). Thus, $c_{\rm p}$ was used directly as the capacitance of the magnetometer, $c_{\rm e}$, for simplicity. The change in inverse capacitance between two

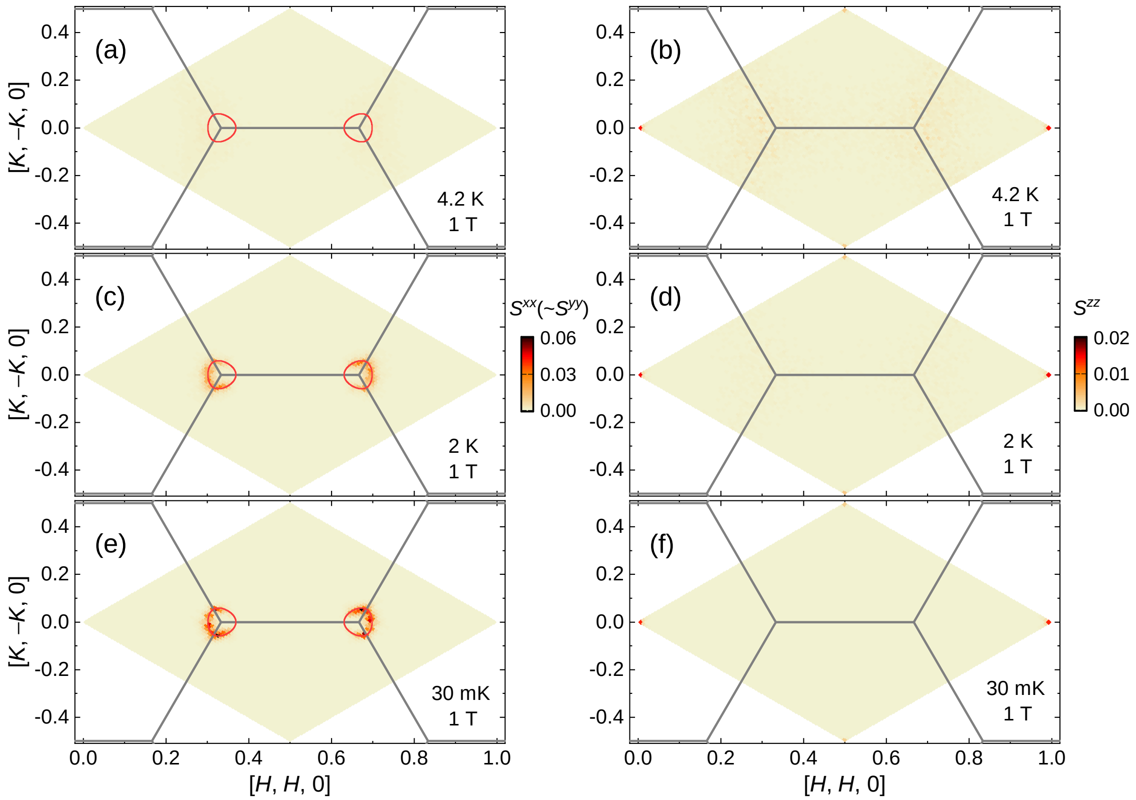


FIG. S4. Spin structure factors $S^{xx}$ ($\sim S^{yy}$) [(a), (c), (e)] and $S^{zz}$ [(b), (d), (f)] calculated at $\mu_0 H^{\parallel}$ = 1 T. Red lines represent the spiral contour [Eq. (8)], and grey lines denote Brillouin zone boundaries. Panels (a), (c), and (e) for $S^{xx}$ share the same scale, as do panels (b), (d), and (f) for $S^{zz}$.

different gradients (e.g., $-10$ and 10 T/m) is given by

$$\Delta(\frac{1}{c_{\mathrm{e}}}) = M^{\parallel}\frac{\mu_0\mu_{\mathrm{B}}N}{k_{\mathrm{eff}}\epsilon_0 A}\Delta(\frac{\mathrm{d}H^{\parallel}}{\mathrm{d}z}) \propto M^{\parallel}, \tag{3}$$

where $\epsilon_0$ is the vacuum permittivity, $A$ is the area of the polar plate, $k_{\mathrm{eff}}$ is the effective spring coefficient in Hooke's law, and $N$ is the number of $Gd^{3+}$ spins. Scaling to $M^{\parallel}$ measured by PPMS, $k_{\mathrm{eff}} \sim 1.7$ kN/m was obtained below $\sim 1.9$ K for the magnetometer.

## II. SPIRAL SPIN-LIQUID ANSATZ

The combined Monte Carlo (MC) fit suggests that the spin Hamiltonian of GdZnPO can be approximated as

$$\mathcal{H} = J_1 \sum_{\langle j0,j1\rangle} \mathbf{S}_{j0}\cdot\mathbf{S}_{j1} + J_2 \sum_{\langle\langle j0,j2\rangle\rangle} \mathbf{S}_{j0}\cdot\mathbf{S}_{j2} + D\sum_{j0}(S^z_{j0})^2 - \mu_0 H^{\parallel} g\mu_{\mathrm{B}} \sum_{j0} S^z_{j0}, \tag{4}$$

where $J_1 \sim -0.39$ K and $J_2 \sim 0.57$ K are the first- ($\langle\ \rangle$) and second- ($\langle\langle\ \rangle\rangle$) nearest-neighbor couplings, respectively, and $D \sim 0.30$ K represents an easy-plane anisotropy. These interactions lead to spin frustration on the honeycomb lattice. The ground-state phase is expected to be a spiral spin liquid (SSL), with spin vectors on the $A$ and $B$ sublattices given by [11]

$$\mathbf{S}_A = S[\cos\psi\cos(\mathbf{Q}\cdot\mathbf{R}), \cos\psi\sin(\mathbf{Q}\cdot\mathbf{R}), \sin\psi] \quad \text{and} \tag{5}$$

$$\mathbf{S}_B = S[\cos\psi\cos(\mathbf{Q}\cdot\mathbf{R}+\phi), \cos\psi\sin(\mathbf{Q}\cdot\mathbf{R}+\phi), \sin\psi], \tag{6}$$

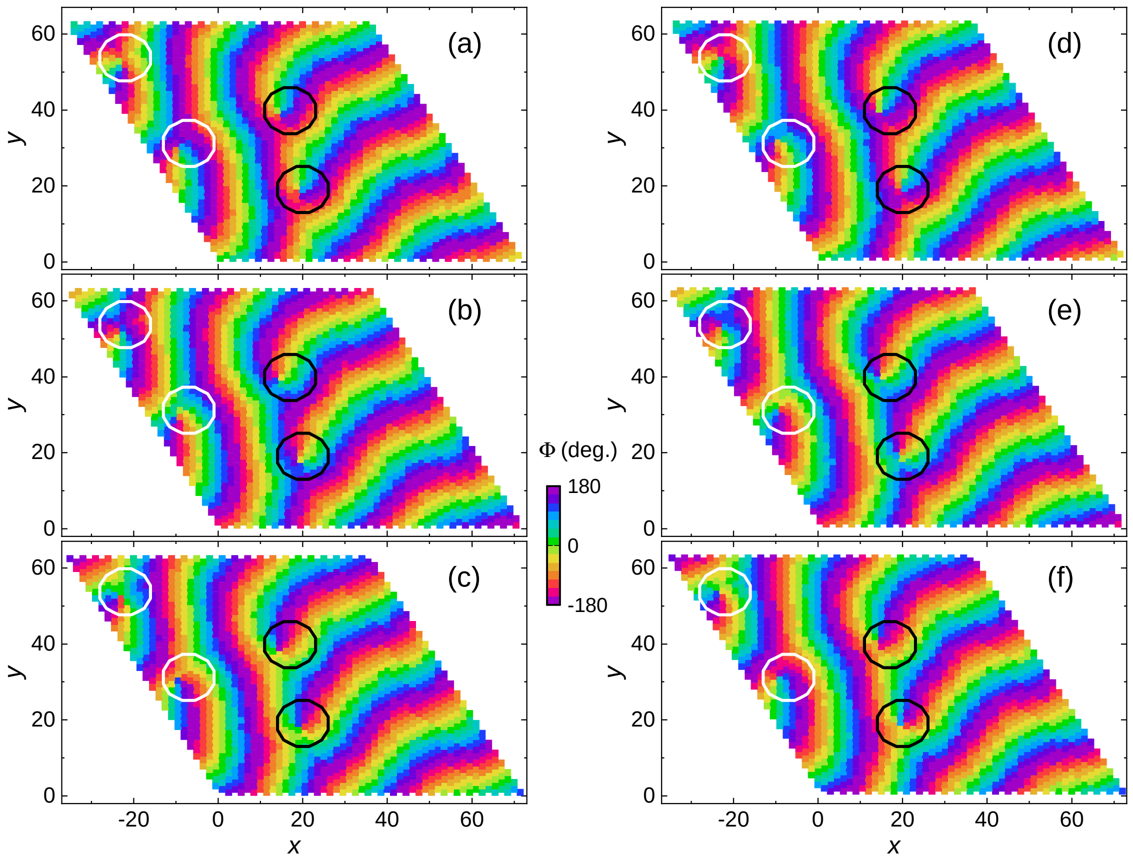


FIG. S5. Spin configuration projected onto the $ab$ plane, $\Phi = -i\ln\frac{S^x+iS^y}{\sqrt{(S^x)^2+(S^y)^2}}$, calculated at 30 mK and $\mu_0 H^{\parallel}$ = 1 T for sublattices $A$ I (a), $A$ II (b), $A$ III (c), $B$ I (d), $B$ II (e), and $B$ III (f). White and black circles indicate spin vortices and antivortices, respectively. All panels share the same $\Phi(\mathbf{r})$ scale, with highlighted vortex and antivortex loops unchanged across panels.

where $\mathbf{R}$ is the unit cell position, $\mathbf{Q} = h\mathbf{b}_1 + k\mathbf{b}_2$ is the ordering wave vector, and $\mathbf{b}_1$, $\mathbf{b}_2$ are reciprocal lattice vectors. The energy per site is given by

$$E = (D + \frac{3J_1}{2} + 3J_2)S^2\sin^2\psi + h_Z S\sin\psi + \frac{J_1 S^2\cos^2\psi}{2}[\cos\phi + \cos(\phi - 2\pi h) + \cos(\phi - 2\pi h - 2\pi k)] + J_2 S^2\cos^2\psi[\cos(2\pi h) + \cos(2\pi k) + \cos(2\pi h + 2\pi k)], \quad (7)$$

where $h_Z = -\mu_0 H^{\parallel} g\mu_B$. Minimizing this expression, we find $\cos\phi = \frac{f_1}{\sqrt{f_1^2+f_2^2}}$, $\sin\phi = \frac{f_2}{\sqrt{f_1^2+f_2^2}}$, and $\sin\psi = -\frac{h_Z}{2S\eta}$, where $f_1 = 1 + \cos(2\pi h_G) + \cos(2\pi h_G + 2\pi k_G)$, $f_2 = \sin(2\pi h_G) + \sin(2\pi h_G + 2\pi k_G)$, and $\eta = D + \frac{3J_1}{2} + \frac{9J_2}{2} + \frac{J_1^2}{8J_2}$. The spiral contour is given by

$$\cos(2\pi h_G) + \cos(2\pi k_G) + \cos(2\pi h_G + 2\pi k_G) = \frac{1}{2}(\frac{J_1^2}{4J_2^2} - 3). \quad (8)$$

Finally, the zero-temperature energy and magnetization are analytically expressed as

$$E_0 = -\frac{h_Z^2}{4\eta} - (\frac{J_1^2}{8J_2} + \frac{3J_2}{2})S^2 \text{ for } |h_Z| \le 2S\eta\text{ , } E_0 = (D + \frac{3J_1}{2} + 3J_2)S^2 + h_Z S \text{ for } |h_Z| > 2S\eta, \quad (9)$$

$$M^{\parallel} = -\frac{h_Z g}{2\eta} \text{ for } |h_Z| \le 2S\eta\text{ , and } |M^{\parallel}| = Sg \text{ for } |h_Z| > 2S\eta. \quad (10)$$

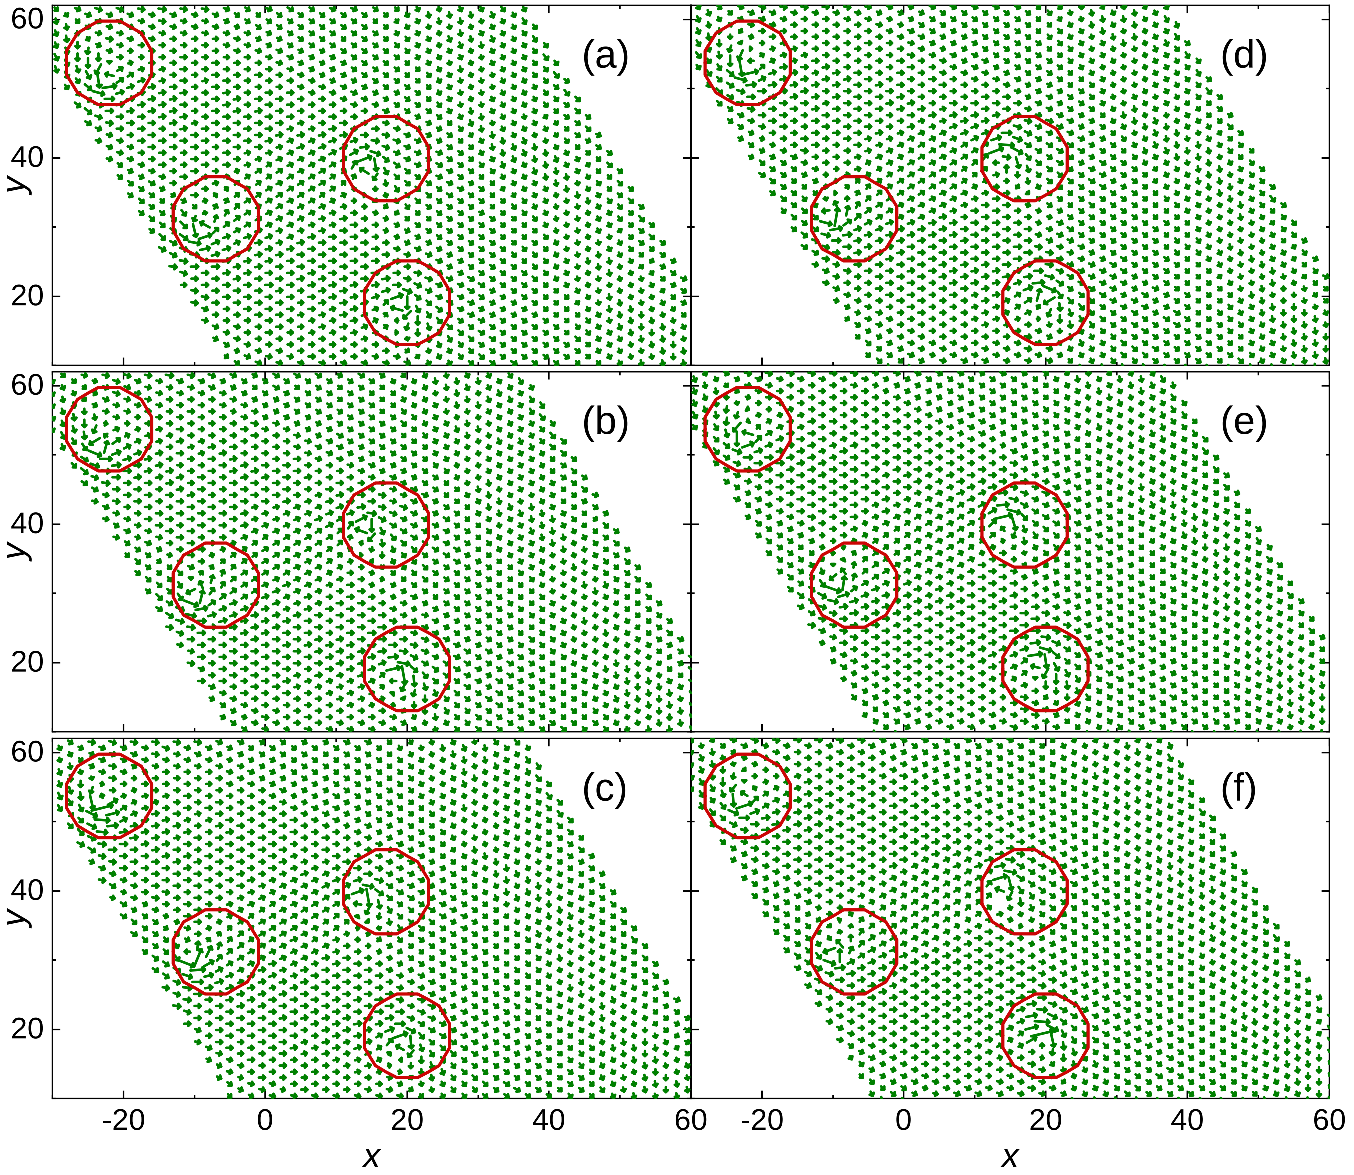


FIG. S6. Sublattice gradient of the spin configuration, $\nabla\Phi(\mathbf{r})$, on sublattices $A$ I (a), $A$ II (b), $A$ III (c), $B$ I (d), $B$ II (e), and $B$ III (f). Local momentum vortices (red circles) appear around the same positions as the topological defects shown in Fig. S5.

## III. MONTE CARLO SIMULATIONS AND LOW-ENERGY TOPOLOGICAL DEFECTS.

We conducted unbiased MC simulations on $2\times L_N^2$ clusters with periodic boundary conditions using the determined spin Hamiltonian of GdZnPO. In Fig. 2 of the main text, we employed an $L_N$ = 9 cluster, averaged over 40 independent samples, to fit the magnetization data above 1.9 K. For Fig. 4 in the main text, we used an $L_N$ = 72 cluster in panel (a), an $L_N$ = 15 cluster averaged over 64 independent samples in panel (b) [also in Fig. 3(b) of the main text], an $L_N$ = 72 cluster averaged over 20 independent samples in panels (c) and (d) (also in Fig. S4), and an $L_N$ = 72 cluster in panels (e) and (f) (also in Figs. S5-S7). Figs. S5-S7 depict the same spin state. A total of 5,000 to 10,000 MC steps were performed, with 500 to 4,000 steps allocated for thermalization. The energy became nearly independent of the number of MC steps after approximately 200 steps, at $T \geq$ 0.03 K.

At 30 mK, the MC energy per spin $E$ agrees well with the analytical energy $E_0$ calculated using Eq. (9) [see Fig. 4(a) in the main text]. More specifically, $E_0$ is consistently lower than $E$ across various magnetic fields, with $E - E_0 \sim$ 0.1 K/spin, supporting the validity of the ground-state ansatz given by Eqs. (5) and (6). Additionally, the low-temperature MC magnetization

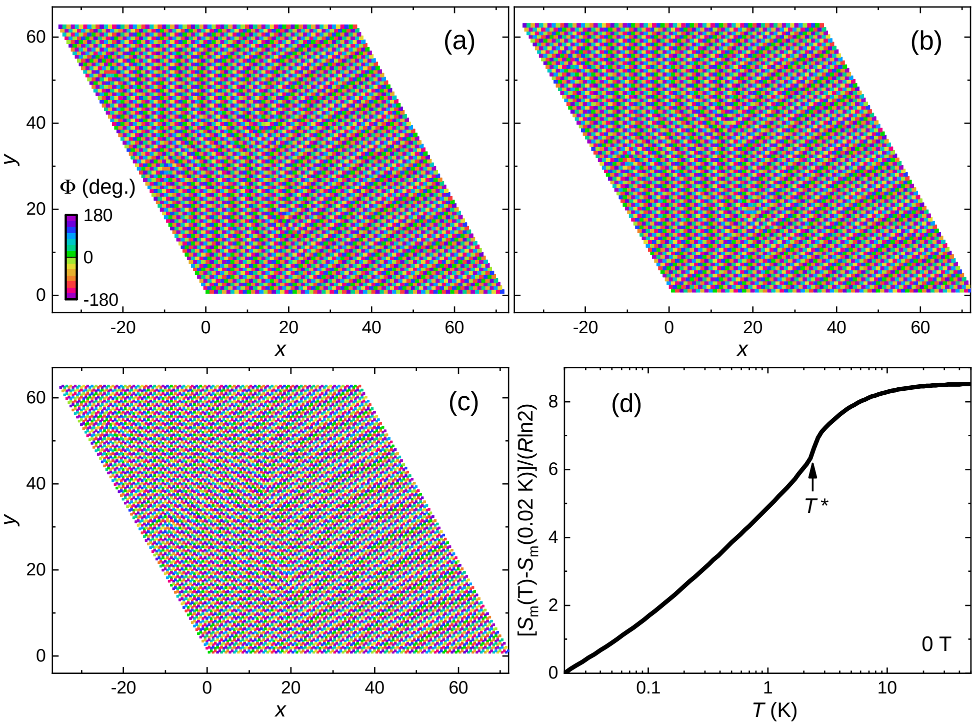


FIG. S7. The spin configuration projected onto the $ab$ plane, $\Phi = -i \ln \frac{S^x + iS^y}{\sqrt{(S^x)^2+(S^y)^2}}$, calculated at 30 mK and $\mu_0 H^{\parallel}$ = 1 T for sublattice $A$ (a), sublattice $B$ (b), and the entire honeycomb lattice (c). Panels (a)-(c) share the same $\Phi(\mathbf{r})$ scale, as shown in panel (a). (d) Entropy increase $S_{\mathrm{m}}(T) - S_{\mathrm{m}}(0.02\ \mathrm{K})$ at 0 T, calculated using classical Monte Carlo simulations, with the crossover temperature $T^*$ indicated.

aligns well with the zero-temperature magnetization predicted by Eq. (10).

The MC specific heat ($C_{\mathrm{m}}$) shows a peak at $T^* \sim 2$ K [see Fig. 4(b) in the main text], which is roughly consistent with the experimental data [see Fig. S2(a)]. To understand the entropy release around $T^*$, we analyzed the spin configurations at various temperatures. At high temperatures (e.g., 50 K, $\gg |J_1|S^2$), the spins exhibit no orientation preference, and $C_{\mathrm{m}}$ remains low, as the average absolute components approach their high-$T$ limits, $\langle|S^{\perp}|\rangle = \langle\sqrt{(S^x)^2 + (S^y)^2}\rangle \to \frac{S}{2}\int_0^{\pi} \sin^2\theta \mathrm{d}\theta$ (= $\frac{\pi S}{4}$) and $\langle|S^z|\rangle \to \frac{S}{2}\int_0^{\pi} \sin\theta|\cos\theta|\mathrm{d}\theta$ (= $\frac{S}{2}$). As the temperature decreases, $\langle|S^{\perp}|\rangle$ approaches 1 and $\langle|S^z|\rangle$ approaches 0 near the specific heat peak, signaling the formation of coplanar spin configurations in the $ab$ plane due to easy-plane anisotropy $D$. This entropy release is primarily attributed to the transition from a three-dimensional spin configuration at higher temperatures to a two-dimensional one as the system cools. Additionally, the transition from a thermally paramagnetic phase to the low-temperature SSL, which spontaneously breaks chiral symmetry at $T^*$ [12], also contributes to the specific heat peak.

We further computed the spin structure factors (Fig. S4),

$$S^{\alpha\alpha}(\mathbf{k}) = \langle|\frac{1}{N}\sum_j S_j^{\alpha} \exp(i\mathbf{k}\cdot\mathbf{R}_j)|^2\rangle,\ \alpha = x, y,\ \text{or}\ z, \tag{11}$$

where $\mathbf{R}_j$ represents the position of the $j$th spin on the honeycomb lattice, $N = 2\times72^2$ = 10,368 is the total number of spins, and $\langle\rangle$ denotes an average over 20 independent samples. Below $T^*$, $S^{xx}$ ($\sim S^{yy}$) exhibits significant intensity around the spiral contour [Eq. (8)], with this intensity increasing as the temperature decreases [compare Figs. S4(e) and S4(c)]. In contrast, $S^{zz}$ shows an intensity of $\sim S^2 \sin^2\psi$ at the $\Gamma$ point, which remains almost constant below $\sim$ 4.2 K [see Figs. S4(b), S4(d), and S4(f)], consistent with the SSL ansatz. For magnetic fields $-h_{\mathrm{Z}}$ between 0 and the saturation value $-h_{\mathrm{Z}}^{\mathrm{s}} = 2S\eta$, the in-plane spin components exhibit incommensurable order, while the out-of-plane components form ferromagnetic order, below $T^*$. Therefore, $T^*$ is also related to the transition between the SSL and thermally paramagnetic phases. Moreover, no clear evidence of "order by disorder" [13, 14] was observed in the MC simulations, down to the lowest experimentally achievable temperature of $\sim$ 30 mK, in agreement with experimental observations (see the main text).

[1] H. Lincke, R. Glaum, V. Dittrich, M. Tegel, D. Johrendt, W. Hermes, M. H. Möller, T. Nilges, and R. Pöttgen, "Magnetic, optical, and electronic properties of the phosphide oxides REZnPO (RE = Y, La-Nd, Sm, Gd, Dy, Ho)," Z. Anorg. Allg. Chem. **634**, 1339 (2008).

[2] Y. Li, S. Bachus, H. Deng, W. Schmidt, H. Thoma, V. Hutanu, Y. Tokiwa, A. A. Tsirlin, and P. Gegenwart, "Partial up-up-down order with the continuously distributed order parameter in the triangular antiferromagnet $TmMgGaO_4$," Phys. Rev. X **10**, 011007 (2020).

[3] B. Li, X. Chen, Y. Zhao, Z. Ma, Z. Wan, and Y. Li, "Proximate Tomonaga-Luttinger liquid in a spin-$1/2$ ferromagnetic XXZ chain compound," Phys. Rev. Mater. **8**, 074410 (2024).

[4] B. Li, Z. Wan, Y. Song, Z. Ma, Y. Zhao, J. Wang, and Y. Li, "Frustrated magnetism of the spin-1 kagome antiferromagnet $\beta$-$BaNi_3(VO_4)_2(OH)_2$," J. Phys.: Condens. Matter **35**, 505801 (2023).

[5] X. Y. Yue, Z. W. Ouyang, J. F. Wang, Z. X. Wang, Z. C. Xia, and Z. Z. He, "Magnetization and ESR studies on $Cu_4(OH)_6FCl$: An antiferromagnet with a kagome lattice," Phys. Rev. B **97**, 054417 (2018).

[6] X. P. Jin, Z. W. Ouyang, X. C. Liu, T. T. Xiao, J. J. Cao, Z. X. Wang, Z. C. Xia, and W. Tong, "Two-sublattice description of the dimer-trimer chain compound $Li_2Cu_5Si_4O_{14}$: High-field magnetization and ESR studies," Phys. Rev. B **104**, 174423 (2021).

[7] Z. Zhang, Y. Cai, J. Kang, Z. Ouyang, Z. Zhang, A. Zhang, J. Ji, F. Jin, and Q. Zhang, "Anisotropic exchange coupling and ground state phase diagram of Kitaev compound YbOCl," Phys. Rev. Res. **4**, 033006 (2022).

[8] Y. Shimizu, Y. Kono, T. Sugiyama, S. Kittaka, Y. Shimura, A. Miyake, D. Aoki, and T. Sakakibara, "Development of high-resolution capacitive Faraday magnetometers for sub-Kelvin region," Rev. Sci. Instrum. **92**, 123908 (2021).

[9] Y. Zhao, Z. Ma, Z. He, H. Liao, Y.-C. Wang, J. Wang, and Y. Li, "Quantum annealing of a frustrated magnet," Nat. Commun. **15**, 3495 (2024).

[10] Y. Li, S. Bachus, B. Liu, I. Radelytskyi, A. Bertin, A. Schneidewind, Y. Tokiwa, A. A. Tsirlin, and P. Gegenwart, "Rearrangement of uncorrelated valence bonds evidenced by low-energy spin excitations in $YbMgGaO_4$," Phys. Rev. Lett. **122**, 137201 (2019).

[11] K. Fujiwara, S. Kitamura, and T. Morimoto, "Thermal Hall responses in frustrated honeycomb spin systems," Phys. Rev. B **106**, 035113 (2022).

[12] C.-J. Huang, J. Q. Liu, and G. Chen, "Spiral spin liquid behavior and persistent reciprocal kagome structure in frustrated van der Waals magnets and beyond," Phys. Rev. Res. **4**, 013121 (2022).

[13] S. Okumura, H. Kawamura, T. Okubo, and Y. Motome, "Novel spin-liquid states in the frustrated Heisenberg antiferromagnet on the honeycomb lattice," J. Phys. Soc. Jpn. **79**, 114705 (2010).

[14] T. Shimokawa, T. Okubo, and H. Kawamura, "Multiple-$q$ states of the $J_1$-$J_2$ classical honeycomb-lattice Heisenberg antiferromagnet under a magnetic field," Phys. Rev. B **100**, 224404 (2019).
